# Supplementary material for: Taylor Dispersion in Thin Liquid Films of Volatile Mixtures: A Quantitative Model for Marangoni Contraction
Source: arXiv:2102.08727 ancillary file (2022-01-31)
Supplement: Supplementary file 1 [file Supplement.pdf]

Supplementary Materials for

# Taylor Dispersion in Thin Liquid Films of Volatile Mixtures: A Quantitative Model for Marangoni Contraction

O. Ramírez-Soto[1] and S. Karpitschka[1]

[1]*Max Planck Institute for Dynamics and Self-Organization (MPI-DS), Am Fassberg 17, 37077 Göttingen*

## I. EXPERIMENTAL METHOD

The microscope coverslips (VWR cover glass class 1, 24 mm × 24 mm size, 170 µm thick) were cleaned with piranha solution (hydrogen peroxide 30%, VWR Chemicals, and sulfuric acid 95%, VWR Chemicals, mixture, volume fraction 1 : 3, respectively) for 20 min in a soda-lime glass staining jar (DWK Life Sciences). Afterwards, the substrates were rinsed five times with fresh water ("Milli-Q" water, resistivity 18 MΩ cm) and were sonicated for 10 min in hot water at ∼ 80 °C, to ensure complete removal of residues from the piranha solution. The substrates were stored in fresh water and used on the day of preparation. The substrates were dried with a nitrogen drying gun immediately before the experiment under a laminar flow hood. The nitrogen was blown parallel to the substrate from the corner opposite of the tweezers that were used to hold the slide. The substrate was kept protected from dust with a glass petri dish during its transfer from the laminar flow hood to the humidity control chamber where the experiment was done.

The binary mixtures for the droplets were composed of water ("Milli-Q") and one of the following carbon diols: Ethylene Glycol (Sigma Aldrich, purity >= 99.5%), 1,2-propanediol (Sigma Aldrich, purity >= 99.5%), 1,2-Butanediol (Sigma Aldrich, purity >= 98%), and 1,2-Hexanediol (Sigma Aldrich, purity 98%). The chemicals were used as received. An analytical balance was used to prepare mixtures of desired mass fraction $0 < \phi < 1$. The mixtures were prepared and stored in piranha cleaned borosilicate glass vials. Polystyrene microspheres (Thermo Fisher Scientific F8809, 0.2 µm diameter, stock solution concentration 2% w/v, excitation/emission maxima = 540/560nm) were added as tracers, with a mass fraction of $7.8 \times 10^{-5}$ of the particle stock solution in the mixture. The mixtures were sonicated in an ultrasonic bath for ∼ 2 min. The mixtures were stored in a low temperature environment (∼ 5 °C) to avoid changes in concentration due to evaporation and were protected from light with aluminum foil. The mixtures were used within the first two days after preparation and were replaced by fresh ones afterwards. Before experiments, the mixtures were sonicated for ∼ 2 min to ensure good dispersal of the particles. The syringes (Hamilton Gastight Series 1700, volume 10 µL) and the needles (Hamilton Removable Needle, small hub, gauge 22s, tip type 3) were cleaned with a series of solvents (ethanol, Carl Roth, purity >= 99.5, and acetone, Sigma Aldrich, purity >= 99.5, ethanol, and water).

During the experiments, a gas mixture of controlled humidity was continuously injected to membrane-separated antechambers in the atmospheric control chamber (aluminum walls, size ∼ 10 cm × 10 cm × 10 cm, Fig. S1). To achieve arbitrary humidities, fluxes of dry nitrogen and nitrogen saturated with water were regulated with mass flow controllers (MKS Instruments Type MF1) to the desired proportion, with a constant total flux of 500 sccm. The membranes connecting the antechambers to the main chamber were made of interwoven fabric (Wilox Hosiery GmbH tight VITAL 40, 88% polyamide, 12% elastane). They spanned almost the entire area of two opposing side walls, minimizing convection in the main chamber while ensuring quick diffusive exchange with the feed gas. Several humidity sensors (Honeywell HIH-4000 Series) provided a measurement of the humidity distribution in the chamber. Whenever changing the humidity conditions, we waited 1 to 5 minutes for equilibration, before injecting a droplet and starting an experiment.

The chamber was mounted on top of an inverted epi-fluorescence microscope (Nikon Eclipse Ti2E) with large field of view (diameter 25 mm in the image plane). A high power white light source (Lumencor SOLA Light Engine) was used for illumination. With a custom fluorescence filter cube (AHF Analysentechnik, transition wavelength 542 nm), the excitation/emission wavelength range of the fluorescent particles was selected. The microscope was equipped with a water immersion objective (Nikon CFI APO LWD 20X WI) with a numerical aperture of 0.95. By matching the immersion medium of the objective with that of the drop, diffraction-limited imaging is achieved even in the bulk of the working medium. This is utterly important for a good $z$-plane selectivity. The focal plane, parallel to the substrate, was moved with the microscope focusing stage in vertical direction to scan the drop at different z-planes in an automated procedure. The time for switching between focal planes was ∼ 100 ms. The full z-scan was on the order of 10 s, shorter than the time scale on which the flow velocities change for a quasi-stationary drop. Successive upward and downward scans were done to check this. A sequence of ∼ 300 frames was recorded for each plane with a high-speed camera (Phantom VEO 4K-L, imaging speed at 600 to 1000 FPS).

Shadowgraphic side-view imaging was performed with a second camera (Point Grey Grasshopper2, imaging speed

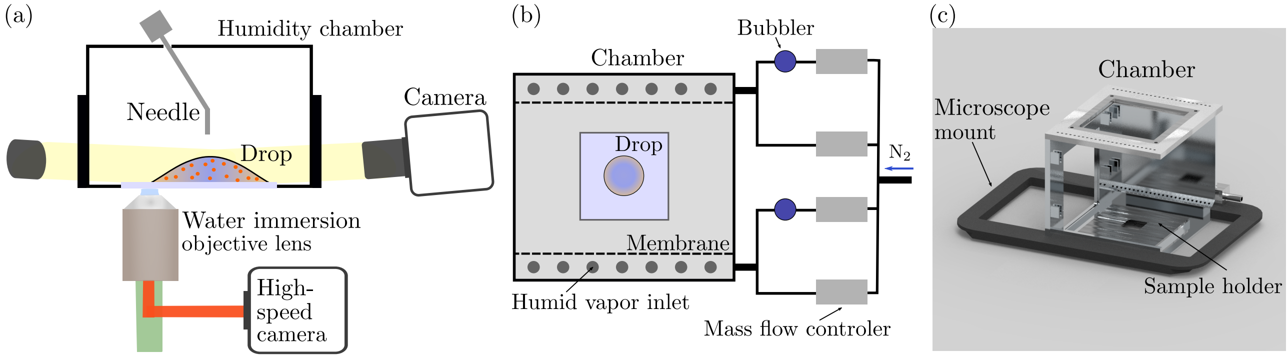


FIG. S1. Experimental setup. (a) Sketch of the experimental setup from side view. (b) Sketch of the humidity chamber and the humidity control system from top view. (c) Inside view of humidity chamber together with microscope mounting system.

at 27 FPS), equipped with a macro lens (Thorlabs Bi-Telecentric lens, 1.0X, W.D. 62.2 mm) and a collimated-light source on the opposite side, both attached to the sample stage of the microscope. The droplets were observed from an angle of 6° with respect to the substrate. The advantage of this arrangement is the possibility of observing the entire three phase contact line around the droplet. This allows for a precise measurement of the footprint diameter of the droplet. The top surface of the drop reflects light directly from the light source to the camera, which allows a precise detection of the drop height, and thereby the apparent contact angle.

## II. CONTACT ANGLE MEASUREMENTS

For each frame from the side-view camera, the droplet's radius $R$ and maximum height $h_0$ were extracted from the images. By assuming that the drop shape is close to a spherical cap, the apparent contact angle was calculated as $\theta_{app} = 2h_0/R$. The images were analyzed with an in-house-developed MATLAB code. The centroid location and the minor and major axes length of the drop are obtained with the regionprops function. The maximum intensity on the short axis corresponds to the top of the drop. For finding the apex position with subpixel resolution, a second order polynomial is fitted to the intensity peak. To calculate $h_0$, the distance from the major axis is measured. The finite observation angle is corrected according to $h_o = h'/cos(\alpha)$, where $\alpha$ is the tilting angle of the side view camera. $R$ is defined as half of the major axis length.

## III. MICRO PARTICLE IMAGE VELOCIMETRY ANALYSIS

For the flow quantification, the images from the PIV measurements were analyzed with an in-house developed code. The data is evaluated through cross-correlation with correlation-averaging over $\sim 100$ frames. The algorithm includes an adaptive interrogation window size method. First, single-pixel correlations are calculated for the entire image and all displacements within a pre-defined search range. Instead of correlating intensity values directly, we used the dot product of the gradient (first order differences). Then, correlations are integrated over interrogation windows of various sizes by convolution with a square kernel of the desired size. We used five different interrogation window sizes of 4, 8, 16, 32, and 64 px side-length. The final correlation maps are then evaluated by a weighted average between the different window sizes, using the mean square of the intensity gradient values in the interrogation window and a size-dependent bias as weight. This method allows for a high resolution in regions of strong velocity gradients, while preventing artifacts from false correlations where particle densities are low. The method was implemented through the Python API of Tensor Flow, to enable fast computation on graphics processing units. Fig. 2 (a) of the main text shows velocity measurements. The insets show velocity fields in two horizontal planes. The velocities shown in the cross section plot were obtained by azimuthally averaging over $\sim 100\,\mu$m. Velocities from different focal planes are shown in Fig.S2 as a function of $d$. The uncertainties of the velocities (colored bands) are estimated using the standard deviation over the weighted interrogation windows.

Whenever the focal plane comes close to the free surface, correlations are picked up preferentially from below the focal plane because there are no particles outside the drop. This leads to a shift in the correlation plane relative to the focal plane. Accordingly, we applied a correction to the z location of the velocity signal relative to the distance from the free surface. To obtain this correction, we estimated the point spread function and the correlation sensitivity

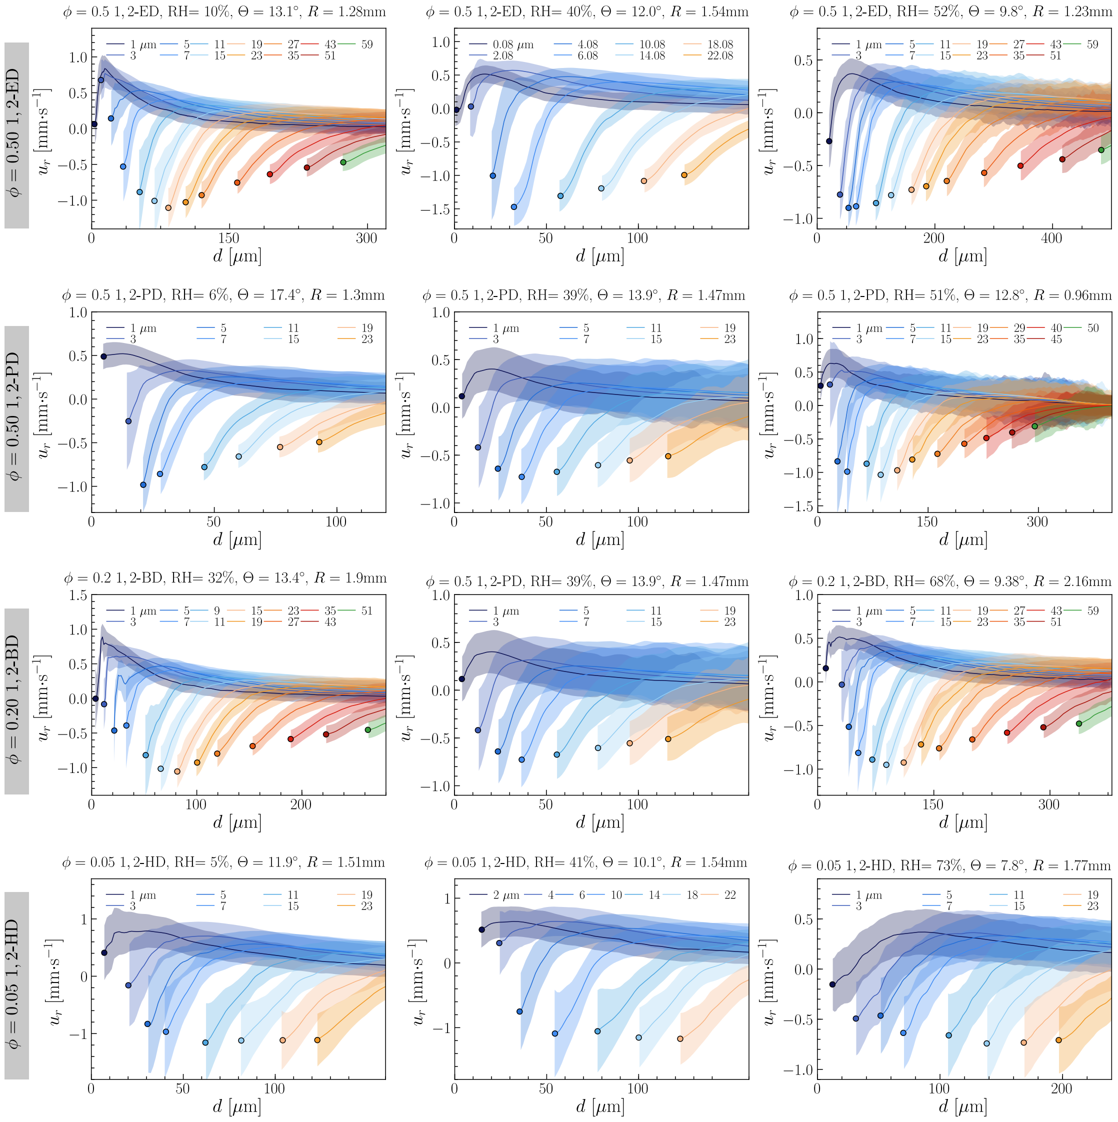


FIG. S2. Radial velocity vs. distance to the contact line for different experimental conditions. Each plot contains the velocities for different z planes above the substrate (solid lines),the associated errors (shaded bands), and the velocities at the interface (circles).

as a function of distance to the focal plane, and convolved this sensitivity with a unit-step function in $z$ for the particle density. For the results shown here, we modeled the depth of correlation as a Gaussian with 1.5 µm standard deviation.

The substrate level was determined at the contact line of the droplet, by focusing onto particles at the substrate. To account for possible substrate tilt and non-planarity, we extracted the expected substrate location from parabolic fits to the velocity profile with a no-slip condition at an offset $z_0$ in the $z$-coordinate. Then we obtained $0 > z_0 \gtrsim 3\,\mu\text{m}$ for $0 < d < 500\,\mu\text{m}$, approximated $z_0(d)$ over the full range of $d$ by a third order polynomial with $z_0(d = 0) = 0$, and used it to correct the vertical substrate location as a function of $d$.

## IV. VELOCITIES AND SURFACE TENSION GRADIENTS

The velocity measurements for a set of experiments with different conditions are presented below. Fig.S3 shows a table with plots for each case. Each row is for one liquid composition and the columns are for different ambient humidity conditions. The title of the plots contain the liquid composition, $\phi$, the relative humidity, RH, the drop

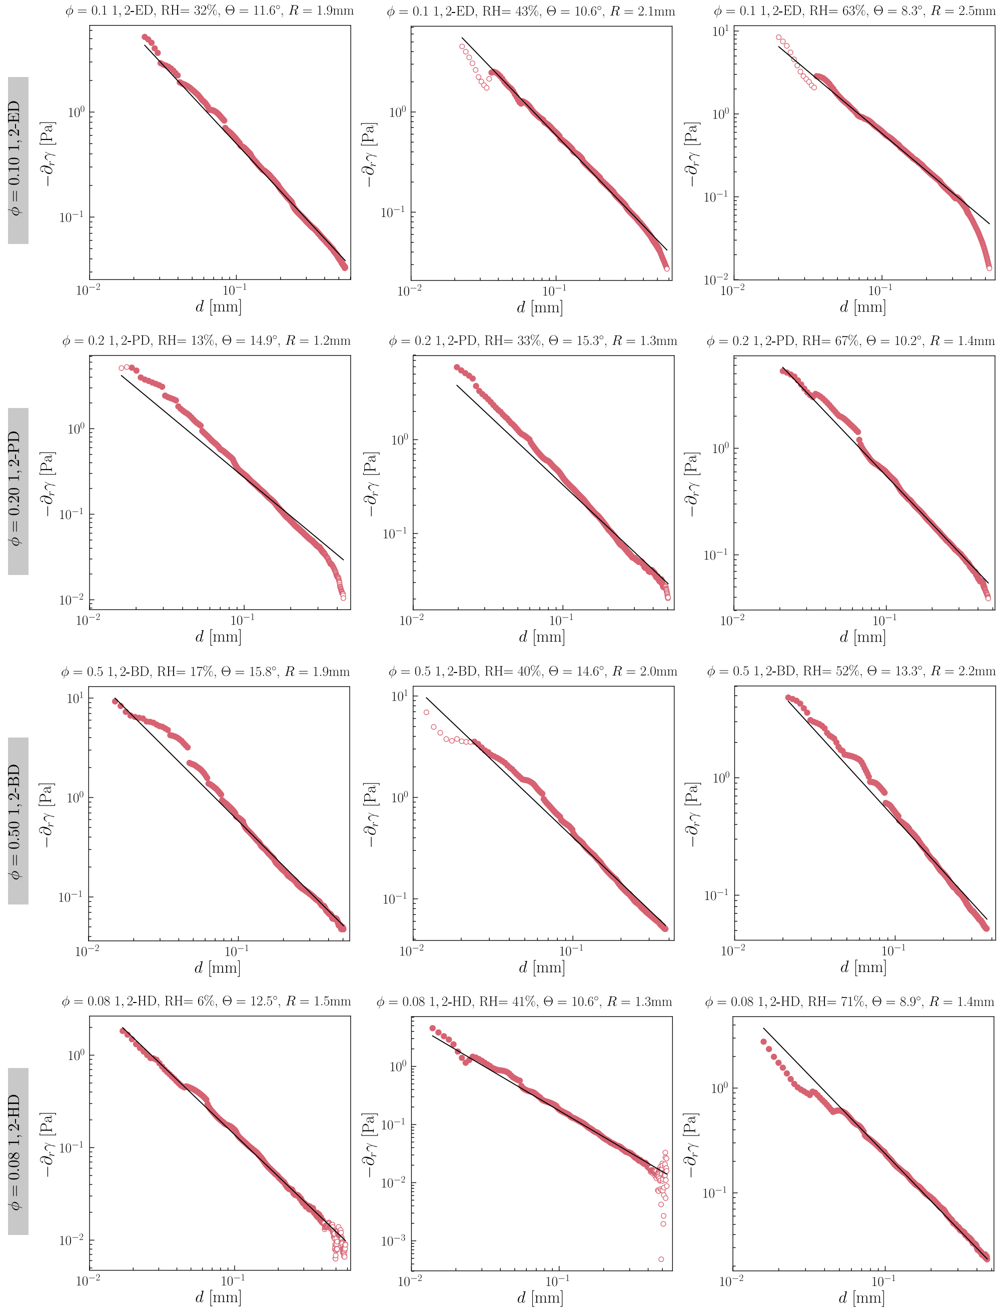


FIG. S3. Surface tension gradient vs. the distance to the contact line. Each plot shows the experimental data (close circles) with the corresponding power law $\partial_r\gamma \sim d^{-3/2}$ (solid lines). The open circles are the data that has not been considered in the fitting.

radius, $R$, and the apparent contact angle $\theta$.

The surface tension gradient was obtained from the first derivative of the velocity profiles in the cross section, evaluated at the interface, and multiplied by the viscosity. The viscosities were interpolated from the data in [1–3]. Fig.S2 shows the surface tension gradient vs. the distance to the contact line for a set of experiments with different conditions. Each plot presents the experimental data (circles), and the power low $\partial_r\gamma \sim d^{-3/2}$ (solid lines).

## V. LUBRICATION THEORY WITH BULK SOLUTES

In absence of bulk solutes, deriving the film height evolution equation in lubrication approximation is a standard procedure that has been done for many situations [4], also including evaporation [5]. Here we introduce our notation, briefly repeat the derivation of the height evolution equation, and systematically extend this formalism for the compositional evolution of bulk solutes.

### A. Problem formulation

We start from incompressible Stokes flow without body forces:

$$\eta\vec{\nabla}^2\vec{u} = \vec{\nabla}p, \tag{S.1}$$

$$\vec{\nabla}\cdot\vec{u} = 0 \tag{S.2}$$

where $\vec{u}$ is the (three-dimensional) fluid velocity field, $\eta$ is the dynamic viscosity of the fluid, and $p$ is the fluid pressure. The evolution of an advected, diffusive solute field $\phi$ (defined as a mass fraction, $\phi \in [0, 1]$) is given by

$$\partial_t\phi = \vec{\nabla}\cdot\left(D\,\vec{\nabla}\phi - \vec{u}\,\phi\right), \tag{S.3}$$

with $t$ as time and $D$ as diffusion coefficient. For simplicity we limit ourselves to the case where the fluid density is independent of $\phi$. We shall also assume that the solute is non-volatile, in contrast to the solvent, which evaporates and has a local mass fraction of $1 - \phi$.

The liquid film shall be limited to $z \in [0, h]$, with a no-slip and no-flux boundary condition at $z = 0$ and a free surface with evaporation and stress boundary conditions at $z = h$:

$$\vec{u}|_{z=0} = 0 \tag{S.4a}$$

$$\vec{u}|_{z=h}\cdot\vec{n} + \vec{j}|_{z=h}\cdot\vec{n} = \vec{n}\cdot\vec{e}_z\,\partial_t h \tag{S.4b}$$

$$\vec{n}\cdot\sigma|_{z=h} = (\gamma\kappa + \Pi)\vec{n} + \vec{\nabla}_s\gamma \tag{S.4c}$$

$$\partial_z\phi|_{z=0} = 0 \tag{S.4d}$$

$$D\,\vec{\nabla}\phi\Big|_{z=h}\cdot\vec{n} = \phi\,\vec{j}|_{z=h}\cdot\vec{n} \tag{S.4e}$$

where $\vec{n}$ shall be the outward surface normal vector at $z = h$, $\vec{j}$ the evaporative flux, expressed in units of volume in the liquid state, $\sigma$ is the fluid stress, $\gamma$ is the surface tension, $\kappa$ is the curvature of the free surface (positive for a convex film surface), $\Pi$ is the disjoining pressure and $\vec{\nabla}_s$ is the surface gradient operator.

The gradient ($\vec{\nabla}$) and divergence ($\vec{\nabla}\cdot$) operators split into vertical and horizontal components, in both cylinder and cartesian coordinates. In the following we use $\vec{\nabla}_{||}\cdot$ and $\vec{\nabla}_{||}$ to denote the horizontal components (parallel to the substrate plane) of divergence and gradient, respectively, to avoid explicit coordinates. The vertical components will be treated explicitly, using $\partial_z$ for derivatives in vertical direction. Similarly, vector fields with the index $_{||}$ refer to the the horizontal vector components only, which may, however, still depend on the vertical coordinate $z$.

As usual in the long-wave expansion, we assume that the film height $h(\vec{r}_{||})$ is a function of the coordinate $\vec{r}_{||}$ in the substrate plane and has small slopes. We define the vertically averaged velocity $\overline{\vec{u}}$, the total hydrodynamic flux $\vec{\Phi}$, the vertically averaged composition $\overline{\phi}$, and the effective solute height $\Psi$ through

$$\vec{\Phi} = \int_0^h dz\,\vec{u}, = \overline{\vec{u}}\,h, \tag{S.5}$$

$$\Psi = \int_0^h dz\,\phi, = \overline{\phi}\,h, \tag{S.6}$$

and the deviations from the average as

$$\vec{u} = \overline{\vec{u}} + \delta\vec{u}, \tag{S.7}$$

$$\phi = \overline{\phi} + \delta\phi. \tag{S.8}$$

Note already that $\delta\vec{u}$ is of the same order as $\overline{\vec{u}}$ while, at some later point, we will require $\delta\phi$ to be small in order to allow for a long-wave description of the composition.

The task is now to derive evolution equations in terms of the vertically averaged quantities alone, taking the limit of long waves i.e., that the characteristic horizontal scale, $r_0$ shall be much larger than the characteristic vertical scale, $h_0$. The aspect ratio,

$$\epsilon_h = \frac{h_0}{r_0} \ll 1, \tag{S.9}$$

will serve as a small parameter. We also define $\delta\phi = \epsilon_\phi\, \delta\phi'$, using $\epsilon_\phi$ as characteristic scale scale of vertical compositional gradients. In the following, we scale all horizontal coordinates as $r = r_0\, r'$, and all vertical coordinates as $h = \epsilon_h\, r_0 h'$. Analogously, horizontal and vertical velocity components are scaled as $\vec{u}_\| = u_0 \vec{u}'_\|$ and $u_z = \epsilon_h u_0 u'_z$, respectively. Time will be scaled as $t = t_0\, t'$ and surface tension as $\gamma = \gamma_0\, \gamma'$, where $\gamma_0 = \gamma(\phi = 0)$ is the surface tension of the pure solvent. The diffusivity $D$ may depend on the local composition $\phi$, so we rescale $D = D_0\, D'$ and define $D' = (1 + \delta D'(\phi))$. Assuming $\partial_\phi \delta D' \lesssim O(1)$, the differences in diffusivity in vertical direction will be small. We also assume that viscosity differences in $z$-direction are negligible. Finally, we scale $j = j_0\, j'$ for the evaporation rate, where $j_0$ will be derived assuming diffusion limited evaporation into an ideal gas atmosphere [5].

$r_0$ and $h_0$ reflect the morphology of the liquid film, while $t_0$ and $u_0$ will be associated with the natural scales that arise from the material properties and the evolution equations. $\gamma_0$, $D_0$, and $j_0$ are material properties. In the following we will omit the primes for readability and work exclusively with scaled quantities, unless stated explicitly.

### B. Hydrodynamic fluxes and height evolution

The vertical integral of Eq. (S.2), together with the kinematic boundary condition (S.4b) and the flux (S.5), yields the evolution equation for thin films:

$$\partial_t h = -\vec{\nabla}_\| \cdot \vec{\Phi}_\| - \mathcal{E}\, j, \tag{S.10}$$

where we have set $t_0 = r_0/u_0 = r_0\, \eta/(\epsilon_h^3 \gamma_0)$, the natural time scale of the hydrodynamic film height evolution, and defined a dimensionless evaporation (Shearwood) number

$$\mathcal{E} = \frac{j_0\, \eta}{\epsilon_h^4\, \gamma_0}. \tag{S.11}$$

Note that Eq. (S.10) does not contain approximations, it fully accounts for volume conservation. All approximations are within the expression that will be used for $\vec{\Phi}_\|$.

Applying the limit $\epsilon_h \ll 1$ to Eq. (S.1), and making use of boundary condition (S.4c), the horizontal components of the velocity are governed by

$$\partial_z^2 \vec{u}_\| = \vec{\nabla}_\| \left( -\gamma \vec{\nabla}_\| \cdot \vec{\nabla}_\| h + \frac{r_0}{\epsilon_h\, \gamma_0}\, \Pi \right) + O(\epsilon_h^2), \tag{S.12}$$

where we have defined $u_0 = \epsilon_h^3\, \gamma_0/\eta$ from the natural scale for the horizontal velocity components i.e., the capillary velocity for horizontal flow in a thin film.

Eq. (S.12) can be integrated to give an explicit expression for $\vec{u}_\|$. The integration constants are determined by the boundary conditions (S.4a) and (S.4c):

$$\vec{u}_\| = \underbrace{\left( \frac{z^2}{2} - h\, z \right) \vec{\nabla}_\| \left( -\gamma \vec{\nabla}_\| \cdot \vec{\nabla}_\| h + \frac{r_0}{\epsilon_h\, \gamma_0}\, \Pi \right)}_{=\vec{u}_C} + \underbrace{\frac{z}{\epsilon_h^2} \vec{\nabla}_\| \gamma}_{=\vec{u}_M} + O(\epsilon_h^2), \tag{S.13}$$

The vertical velocity component follows from Eq. (S.2). The characteristic velocity of vertical flows is therefore $\epsilon_h\, u_0$, much smaller than the horizontal components. The total hydrodynamic flux is given by the integral of Eq. (S.13) over the entire depth of the film:

$$\vec{\Phi}_\| = \underbrace{\frac{h^3}{3} \vec{\nabla}_\| \left( \gamma \vec{\nabla}_\| \cdot \vec{\nabla}_\| h - \frac{r_0}{\epsilon_h\, \gamma_0}\, \Pi \right)}_{=\vec{\Phi}_C} + \underbrace{\frac{1}{\epsilon_h^2} \frac{h^2}{2} \vec{\nabla}_\| \gamma}_{=\vec{\Phi}_M} + O(\epsilon_h^2). \tag{S.14}$$

The horizontal velocity and the total hydrodynamic flux both split up into a pressure-driven (capillary) component $\vec{\Phi}_C$ with a Poiseuille-type velocity profile, and a Marangoni component $\vec{\Phi}_M$ with a Couette-type velocity profile. The velocities can be expressed in terms of the fluxes:

$$\vec{u}_C = 3\left(\frac{z}{h} - \frac{1}{2}\left(\frac{z}{h}\right)^2\right)\frac{\vec{\Phi}_C}{h} + O(\epsilon_h^2), \tag{S.15}$$

$$\vec{u}_M = 2\frac{z}{h}\frac{\vec{\Phi}_M}{h} + O(\epsilon_h^2). \tag{S.16}$$

Therefore, the height evolution equation (S.10) with the horizontal flux from Eq. (S.14) is purely two-dimensional and does not require any $z$-resolved quantities. The profiles of the horizontal velocity components follow from Eqs. (S.15) & (S.16), the vertical velocity from the $z$-integral of Eq. (S.2).

### C. Compositional evolution

Inserting Eqs. (S.7), (S.8) into the evolution equation (S.3), applying our scalings, and explicitly writing horizontal and vertical components gives

$$\partial_t\left(\overline{\phi} + \epsilon_\phi\,\delta\phi\right) = \mathrm{Pe}^{-1}\,\vec{\nabla}_\parallel \cdot D\,\vec{\nabla}_\parallel\left(\overline{\phi} + \epsilon_\phi\,\delta\phi\right) + \frac{\epsilon_\phi}{\epsilon_h^2\mathrm{Pe}}\,\partial_z D\,\partial_z\delta\phi - \vec{u}_\parallel\cdot\vec{\nabla}_\parallel\left(\overline{\phi} + \epsilon_\phi\,\delta\phi\right) - \epsilon_\phi\,u_z\,\partial_z\delta\phi. \tag{S.17}$$

Here we found $\mathrm{Pe} = \frac{r_0^2}{t_0\,D_0} = \frac{u_0\,r_0}{D_0} = \frac{\epsilon_h^3\,r_0\,\gamma_0}{D_0\,\eta}$, the Péclet number for characteristic scales in horizontal direction.

In order to obtain an evolution equation in terms of $\overline{\phi}$ alone, we would like to find an expression without terms containing $\delta\phi$. Thus we integrate Eq. (S.17) in $z$ direction, minding the dependence of $h$ on space and time when changing the order of differentiation and integration:

$$\begin{aligned}\partial_t\int_0^h dz\left(\overline{\phi} + \epsilon_\phi\,\delta\phi\right) - \left(\overline{\phi} + \epsilon_\phi\,\delta\phi(h)\right)\partial_t h = \quad & \mathrm{Pe}^{-1}\,\vec{\nabla}_\parallel\cdot\int_0^h dz\,D\,\vec{\nabla}_\parallel\left(\overline{\phi} + \epsilon_\phi\,\delta\phi\right)\\ & + \mathrm{Pe}^{-1}\left(\frac{\epsilon_\phi}{\epsilon_h^2}\left[D\,\partial_z\delta\phi\right]_0^h - D\,\vec{\nabla}_\parallel\left(\overline{\phi} + \epsilon_\phi\,\delta\phi\right)\Big|_h\cdot\vec{\nabla}_\parallel h\right)\\ & - \int_0^h dz\left(\vec{u}_\parallel\cdot\vec{\nabla}_\parallel\overline{\phi}\right) - \epsilon_\phi\int_0^h dz\left(\vec{u}_\parallel\cdot\vec{\nabla}_\parallel\delta\phi + u_z\,\partial_z\delta\phi\right).\end{aligned} \tag{S.18}$$

The integral on the left-hand side and the integral of the advection of the mean composition can readily be evaluated, using the properties of the $z$-dependence of $\overline{\phi}$, $\delta\phi$ and $\overline{u}_h$. We split the diffusion integral into $\overline{\phi}$ and $\delta\phi$ terms and use the definition $\overline{D} = 1 + \frac{1}{h}\int_0^h dz\,\delta D$ to simplify the former term. The boundary term from diffusion represents the total diffusive fluxes across the film boundaries at $z = 0$ and $z = h$, per horizontal area element. These terms are determined by the boundary conditions (S.4d) and (S.4e), where we use the shorthand $j = \frac{\vec{j}(h)\cdot\vec{n}}{\vec{n}\cdot\vec{e}_z}$. On the $z$-component of the advection of $\delta\phi$ we perform integration by parts, and apply continuity equation (S.2) to the resulting term. Then, the integrand can be combined to a single divergence. The evolution equation reduces to

$$\begin{aligned}h\,\partial_t\overline{\phi} - \epsilon_\phi\,\delta\phi(h)\,\partial_t h = \quad & \mathrm{Pe}^{-1}\,\vec{\nabla}_\parallel\cdot\left(\overline{D}\,h\,\vec{\nabla}_\parallel\overline{\phi} + \epsilon_\phi\int_0^h dz\,D\,\vec{\nabla}_\parallel\delta\phi\right) + \mathcal{E}\left(\overline{\phi} + \epsilon_\phi\,\delta\phi(h)\right)j\\ & - \vec{\Phi}\cdot\vec{\nabla}_\parallel\overline{\phi} - \epsilon_\phi\left[u_z\,\delta\phi\right]_0^h + \epsilon_\phi\int_0^h dz\left(\vec{\nabla}_\parallel\cdot\delta\phi\,\vec{u}_\parallel\right).\end{aligned} \tag{S.19}$$

On the last term, we change the order of differentiation and integration once more:

$$\begin{aligned}h\,\partial_t\overline{\phi} - \underline{\epsilon_\phi\,\delta\phi(h)\,\partial_t h} = \quad & \mathrm{Pe}^{-1}\,\vec{\nabla}_\parallel\cdot\left(\overline{D}\,h\,\vec{\nabla}_\parallel\overline{\phi} + \epsilon_\phi\int_0^h dz\,D\,\vec{\nabla}_\parallel\delta\phi\right) + \mathcal{E}\left(\overline{\phi} + \epsilon_\phi\,\delta\phi(h)\right)j\\ & - \vec{\Phi}\cdot\vec{\nabla}_\parallel\overline{\phi} - \underline{\epsilon_\phi\left(\left[u_z\,\delta\phi\right]_0^h - \delta\phi\,\vec{u}_\parallel\big|_h\cdot\vec{\nabla}_\parallel h\right)} - \epsilon_\phi\,\vec{\nabla}_\parallel\cdot\int_0^h dz\,\delta\phi\,\vec{u}_\parallel,\end{aligned} \tag{S.20}$$

As in the evolution equation for $h$, we make use of the boundary conditions (S.4a) and (S.4b), to show that the underlined terms in the equation above cancel. This leads to

$$h\,\partial_t\overline{\phi} = \mathrm{Pe}^{-1}\,\vec{\nabla}_{\|}\cdot\left(\overline{D}\,h\,\vec{\nabla}_{\|}\overline{\phi} + \epsilon_\phi\int_0^h dz\,D\,\vec{\nabla}_{\|}\delta\phi\right) + \mathcal{E}\left(\overline{\phi}+\epsilon_\phi\,\delta\phi(h)\right)j - \vec{\Phi}\cdot\vec{\nabla}_{\|}\overline{\phi} - \epsilon_\phi\,\vec{\nabla}_{\|}\cdot\int_0^h dz\,\delta\phi\,\vec{u}_{\|}. \tag{S.21}$$

Note that in deriving Eq. (S.21) from Eq. (S.3), no approximations have been made.

The integral of the continuity equation for velocity, Eq. (S.10), which is also exact apart from the expression used for $\vec{\Phi}_{\|}$, can be formulated solely in terms of the vertical integral of velocity, $\vec{\Phi}_{\|}$. This is not the case for Eq. (S.21), which still contains terms with $\delta\phi$. In order to derive an evolution equation in terms of $\overline{\phi}$ alone, approximations must be made. Importantly, the expression that we intend to use for $\vec{\Phi}_{\|}$ (Eq. (S.14)) in Eq. (S.10) is precise up to terms of $O(\epsilon_h^2)$. Thus an analog equation for the evolution of $\overline{\phi}$ should retain any terms of $O(\epsilon_h)$ in order to be consistent with Eqs. (S.10) and (S.14).

The approximate evolution equation for $\overline{\phi}$ depends on the magnitude of $\epsilon_\phi$, which will be determined later. In the case that $\epsilon_\phi$ is not small, typically a simple evolution equation in terms of $\overline{\phi}$ cannot be derived. Then the full advection-diffusion problem has to be solved. Thus we now implement a first (mild) approximation that requires $\epsilon_\phi \ll 1$ and $\partial_\phi\delta D = O(1)$, in order to remove the $z$-dependence of the diffusivity. Then, $\overline{D} \lesssim 1 + \delta D(\overline{\phi}) + O(\epsilon_\phi)$ and $D = \overline{D} + O(\epsilon_\phi)$. Further we assume $\mathcal{E} \ll 1$, which is the case for our droplets, to eliminate $\delta\phi$ from the evaporation term. This simplifies Eq. (S.21) to

$$h\,\partial_t\overline{\phi} = \mathrm{Pe}^{-1}\,\vec{\nabla}_{\|}\cdot\left(\overline{D}\,h\,\vec{\nabla}_{\|}\overline{\phi} - \epsilon_\phi\,\overline{D}\,\delta\phi(h)\,\vec{\nabla}_{\|}h\right) + \mathcal{E}\,\overline{\phi}\,j - \vec{\Phi}\cdot\vec{\nabla}_{\|}\overline{\phi} - \epsilon_\phi\,\vec{\nabla}_{\|}\cdot\int_0^h dz\,\delta\phi\,\vec{u}_{\|} + O(\epsilon_\phi^2). \tag{S.22}$$

In the following we will examine various limits and the resulting evolutions equations for the composition.

*Limit I — $\epsilon_\phi \ll \epsilon_h$*

If $\epsilon_\phi$ turns out to be exceedingly small i.e., $\epsilon_\phi\,\delta\phi \ll \epsilon_h$, vertical gradients in the composition are fully suppressed, and the governing equation simply becomes an advection-diffusion equation in terms of the vertically averaged quantities alone:

$$\underline{\epsilon_\phi \ll \epsilon_h}: \qquad h\,\partial_t\overline{\phi} = \mathrm{Pe}^{-1}\,\vec{\nabla}_{\|}\cdot\overline{D}\,h\,\vec{\nabla}_{\|}\overline{\phi} - \vec{\Phi}_{\|}\cdot\vec{\nabla}_{\|}\overline{\phi} + \mathcal{E}\,\overline{\phi}\,j. \tag{S.23}$$

This equation has been used in the existing literature and properly accounts for mass conservation and evaporation in a diffusion dominated problem. Dispersion terms are missing.

*Limit II — $\epsilon_\phi \sim \epsilon_h$*

If we assume $\epsilon_\phi \sim \epsilon_h \ll 1 \ll \mathrm{Pe}$, which is the case when advection dominates the horizontal transport, the leading order problem reduces to advection and evaporation alone. To be consistent with the order of Eq. (S.10) with Eq. (S.14), we should keep terms of $O(\epsilon_\phi)$ and $O(\mathrm{Pe}^{-1})$ that account for diffusion and dispersion, but drop terms of $O(\epsilon_\phi\mathrm{Pe}^{-1})$ or higher:

$$h\,\partial_t\overline{\phi} = \mathrm{Pe}^{-1}\,\vec{\nabla}_{\|}\cdot\overline{D}\,h\,\vec{\nabla}_{\|}\overline{\phi} + \mathcal{E}\,\overline{\phi}\,j - \vec{\Phi}\cdot\vec{\nabla}_{\|}\overline{\phi} - \epsilon_\phi\,\vec{\nabla}_{\|}\cdot\int_0^h dz\,\delta\phi\,\vec{u}_{\|}. \tag{S.24}$$

Next we will show that, consistent with the order-of-magnitude assumptions of limit II, $\delta\phi$ is determined by a governing equation in terms of the averaged composition alone. Thus a closed evolution equation of $\overline{\phi}$ can be derived, with additional terms that describe Taylor dispersion for the general case of a thin free surface film with capillary and Marangoni flows.

The difference between the original advection-diffusion equation and its vertical integral will provide a governing equation for $\delta\phi$. Thus we apply the same approximations to Eq. (S.17), multiply it with $h$, and subtract Eq. (S.24):

$$\begin{aligned}\epsilon_\phi\,h\,\partial_t\delta\phi = \;& \mathrm{Pe}^{-1}\,\vec{\nabla}_{\|}\cdot\overline{D}\vec{\nabla}_{\|}\overline{\phi}\cdot\vec{\nabla}_{\|}h - h\,\delta\vec{u}_{\|}\cdot\vec{\nabla}_{\|}\overline{\phi} - \mathcal{E}\,\overline{\phi}\,j + \frac{\epsilon_\phi}{\epsilon_h^2\mathrm{Pe}}\,\overline{D}\,h\,\partial_z^2\delta\phi \\ & - \epsilon_\phi\left(h\,\vec{u}_{\|}\cdot\vec{\nabla}_{\|}\delta\phi - h\,u_z\,\partial_z\delta\phi + \vec{\nabla}_{\|}\cdot\int_0^h dz\,\delta\phi\,\vec{u}_{\|}\right),\end{aligned} \tag{S.25}$$

Since the remaining term with $\delta\phi$ in Eq. (S.24) scales as $\epsilon_\phi$, it is sufficient to determine $\delta\phi$ at $O(1)$. Higher order terms in $\delta\phi$ would be of $O(\epsilon^2)$ when inserted into (S.24). Thus, the governing equation for $\delta\phi$ simplifies to

$$\frac{\epsilon_\phi}{\epsilon_h^2\,\mathrm{Pe}}\,\overline{D}\,\partial_z^2\delta\phi = \mathcal{E}\,\frac{\overline{\phi}\,j}{h} + \delta\vec{u}_\parallel\cdot\vec{\nabla}_\parallel\overline{\phi} + O(\epsilon_\phi). \tag{S.26}$$

No explicit time derivative of $\delta\phi$ appears anymore. Rather, $\delta\phi$ appears only in terms of its second vertical derivative. The advection term contains only $\delta\vec{u}_\parallel$, the difference from the depth-averaged velocity. Therefore, Eq. (S.26) represents a stationary advection-diffusion problem in the co-moving frame of the mean flow and can be integrated. This yields an expression for $\delta\phi$ that depends only on the averaged composition and the local evaporation rate. The appropriate choice for $\epsilon_\phi$ now becomes obvious and depends on the relative dominance of the right hand side terms of Eq. (S.25). In our case, $\mathcal{E}\ll 1$ while $\delta\vec{u}_\parallel = O(1)$, so we define $\epsilon_\phi$ from the advection term:

$$\epsilon_\phi = \epsilon_h^2\mathrm{Pe} = \frac{h_0^2\,u_0}{D_0\,r_0}, \tag{S.27}$$

which is equivalent to a Péclet number defined for the characteristic vertical scales [6]. The important feature that allows for above simplifications is identical to that for pipe flow: the aspect ratio $\epsilon_h$ must be small, such that $\epsilon_h^2\mathrm{Pe}\,\delta\phi\ll 1$, while $\mathrm{Pe}\gg 1$. With this definition, Eq. (S.26) becomes (dropping the $O(\epsilon_\phi)$ from now on):

$$\overline{D}\,\partial_z^2\delta\phi = \mathcal{E}\frac{\overline{\phi}\,j}{h} + \delta\vec{u}_\parallel\cdot\vec{\nabla}_\parallel\overline{\phi}. \tag{S.28}$$

Integrating Eq. (S.28) twice from 0 to $z$ gives

$$\overline{D}\,[\delta\phi]_0^z = \mathcal{E}\frac{\overline{\phi}\,j}{h}\frac{z^2}{2} + \vec{\nabla}_\parallel\overline{\phi}\cdot\int_0^z dz'\int_0^{z'} dz''\,\delta\vec{u}_\parallel(z''). \tag{S.29}$$

The integration constant $\delta\phi|_{z=0}$ can be determined by integrating above expression over the entire film height and the vanishing mean of $\delta\phi$:

$$-\overline{D}\,\delta\phi|_{z=0} = \mathcal{E}\frac{h\,\overline{\phi}\,j}{6} + \frac{1}{h}\vec{\nabla}_\parallel\overline{\phi}\cdot\int_0^h dz\int_0^z dz'\int_0^{z'} dz''\,\delta\vec{u}_\parallel(z''). \tag{S.30}$$

$\delta\vec{u}_\parallel$ and its integrals can be expressed in terms of capillary and Marangoni fluxes as derived in the previous section, so the integrals can be evaluated:

$$\overline{D}\,\delta\phi = \mathcal{E}\frac{\overline{\phi}\,j}{h}\left(\frac{z^2}{2}-\frac{h^2}{6}\right) + \vec{\nabla}_\parallel\overline{\phi}\cdot\left(\left(\frac{z^3}{2h}-\frac{z^4}{8h^2}-\frac{z^2}{2}+\frac{h^2}{15}\right)\frac{\vec{\Phi}_C}{h} + \left(\frac{z^3}{3h}-\frac{z^2}{2}+\frac{h^2}{12}\right)\frac{\vec{\Phi}_M}{h}\right). \tag{S.31}$$

Since in this general case, $\delta\phi$ depends on the local film thickness and the fluxes, it is not possible to assess the validity of limit ii solely by the magnitude of $\epsilon_\phi$, which is given by the natural scales. In wetting problems, it is a common observation that the dimensionless fluxes remain much smaller than 1. The same holds for the dimensionless $h$ of a droplet, where the characteristic height is chosen at the apex of the drop. Thus, one expects $\delta\phi\ll 1$, which is the case also for Marangoni contracted droplets. Thus the criterion for limit ii should be revised to $\epsilon_\phi\,\delta\phi\sim\epsilon_h\ll 1\ll\mathrm{Pe}$.

The (Taylor) dispersive flux in evolution equation (S.24) is

$$\begin{aligned}\vec{\Phi}_T = \epsilon_\phi\int_0^h dz\,\delta\phi\,\vec{u}_\parallel = -\epsilon_h^2\mathrm{Pe}\frac{h}{\overline{D}}\Bigg(&\left(\frac{2}{105}\vec{\nabla}_\parallel\overline{\phi}\cdot\vec{\Phi}_C + \frac{1}{40}\vec{\nabla}_\parallel\overline{\phi}\cdot\vec{\Phi}_M - \frac{7}{120}\mathcal{E}\,\overline{\phi}\,j\right)\vec{\Phi}_C \\ &+\left(\frac{1}{40}\vec{\nabla}_\parallel\overline{\phi}\cdot\vec{\Phi}_C + \frac{1}{30}\vec{\nabla}_\parallel\overline{\phi}\cdot\vec{\Phi}_M - \frac{1}{12}\mathcal{E}\,\overline{\phi}\,j\right)\vec{\Phi}_M\Bigg).\end{aligned} \tag{S.32}$$

The evolution equation for $\overline{\phi}$ finally reads

$$\underline{\epsilon_\phi\,\delta\phi\sim\epsilon_h\ll 1\ll\mathrm{Pe}}:\qquad h\,\partial_t\overline{\phi} = \mathrm{Pe}^{-1}\,\vec{\nabla}_\parallel\cdot\overline{D}\,h\,\vec{\nabla}_\parallel\overline{\phi} - \vec{\Phi}_\parallel\cdot\vec{\nabla}_\parallel\overline{\phi} + \mathcal{E}\,\overline{\phi}\,j - \vec{\nabla}_\parallel\cdot\vec{\Phi}_T. \tag{S.33}$$

With radial or translational symmetry, the compositional gradient and the hydrodynamic fluxes are necessarily parallel. This, together with the assumption of a small evaporation rate allows for the following simplifications on $\vec{\Phi}_T$:

$$\vec{\Phi}_T = -\epsilon_h^2\mathrm{Pe}\frac{h}{\overline{D}}\left(\frac{2\vec{\Phi}_C^2}{105} + \frac{\vec{\Phi}_C\cdot\vec{\Phi}_M}{20} + \frac{\vec{\Phi}_M^2}{30}\right)\vec{\nabla}_\parallel\overline{\phi}. \tag{S.34}$$

By defining an effective diffusivity

$$\overline{D}_{\text{eff}} = \overline{D} + \frac{\epsilon_h^2 \mathrm{Pe}^2}{\overline{D}} \left( \frac{2\vec{\Phi}_C^2}{105} + \frac{\vec{\Phi}_C \cdot \vec{\Phi}_M}{20} + \frac{\vec{\Phi}_M^2}{30} \right), \tag{S.35}$$

the Taylor-dispersive flux can then be included in the diffusion term, which leads to the evolution equation

$$\underline{\epsilon_\phi\, \delta\phi \sim \epsilon_h \ll 1 \ll \mathrm{Pe}, \quad \text{2D or axisymmetric}}: \qquad h\, \partial_t \overline{\phi} = \mathrm{Pe}^{-1}\, \vec{\nabla}_{\|} \cdot \overline{D}_{\text{eff}}\, h\, \vec{\nabla}_{\|} \overline{\phi} - \vec{\Phi}_{\|} \cdot \vec{\nabla}_{\|} \overline{\phi} + \mathcal{E}\, \overline{\phi}\, j. \tag{S.36}$$

*Limit III — $\epsilon_\phi \gg \epsilon_h$*

In this case, an evolution equation in terms of the averaged quantities alone cannot be derived.

## SIMULATIONS

We include quasi-stationary diffusion limited evaporation into our simulations by closely following the approach from [5]: We assume that the macroscopic drop body is surrounded by a wetting precursor that is subject to a disjoining pressure and in equilibrium with the vapor above the substrate. Therefore, the local evaporation rate $j$ is calculated by an integral transform of the local vapor pressure $p_v$ of the liquid, which is subject to Raoult's law and Kelvin's law (in physical units):

$$p_v = p_v^{(0)}\, x\, \exp\left( \frac{M\, p}{\rho\, R_g\, T} \right), \tag{S.37}$$

where $p_v^{(0)}$ is the saturation vapor pressure of the pure solvent at atmospheric pressure, $x$ is the mole fraction of the solvent in the mixture, $M$ is the molar mass of the solvent molecule, $\rho$ is the liquid density, $R_g$ is the gas constant and $T$ is the temperature. In contrast to [5], we do not linearize around $p = 0$ to preserve the non-negativity property of Eq. (S.37). While the overall evolution does not seem to be influenced significantly by this, it gives physical vapor pressures also in regions with large negative pressures (i.e., the transition from the drop to the precursor).

As disjoining pressure, we use the standard long-range van-der-Waals form $\Pi = -\gamma_0 a^2/h^3$ (in physical units), where $a^2 = A/\gamma_0$ is a molecular length scale and $A$ is the Hamaker constant [5]. For simplicity we assume that the disjoining pressure is independent of composition. The effect of composition-dependent surface forces in wetting scenarios has been analyzed in the literature [7], but is beyond scope here. In scaled units, the pressure reads

$$p = -\gamma(\phi)\, \partial_r^2 h - \frac{a^2\, r_0^2}{h_0^4}\, \frac{1}{h^3}, \tag{S.38}$$

where we have set $p_0 = \frac{\gamma_0 h_0}{r_0^2}$ from the capillary term. To find a set of dimensionless scales for our simulations, we require the pressure term to be parameter-free, which defines

$$r_0 = \frac{h_0^2}{a}. \tag{S.39}$$

We define the characteristic vertical scale $h_0$ from the liquid-vapor equilibrium of the precursor according to the Kelvin law [5]:

$$\ln \frac{p_v}{p_v^{(0)}} = \frac{M}{\rho\, R_g\, T}\, p_0\, \Pi = -\frac{M}{\rho\, R_g\, T}\, \frac{\gamma_0\, a^2}{h_0^3}\, \frac{1}{h^3}, \tag{S.40}$$

finding

$$h_0 = \left( \frac{\rho\, R_g\, T}{\gamma_0\, a^2\, M} \right)^{1/3}. \tag{S.41}$$

With typical values of the material parameters, $h_0 \sim 0.7\,\text{nm}$ and $r_0 \sim 1.2\,\text{nm}$. In contrast, typical initial droplet heights are $\sim 0.1\,\text{mm}$, radii $1\,\text{mm}$. This strong separation of scaled leads to exceedingly small time steps and long

run times of the simulations. We accelerate the simulations by choosing $h_0$ five times larger than its natural value. According to (S.39), this increases $r_0$ by a factor of 25. We also tested increasing $h_0$ by a factor of 10 or 20, and no significant differences were noticeable.

The physical conservation law in the problem is the conservation of mass for either chemical species, rather than the total volume or the local mass fraction. Thus we cast the evolution equations into the conserved variables $\Psi_i$, the amount of material $i$ per unit substrate area:

$$\Psi_1 = (1 - \overline{\phi})\, h, \tag{S.42a}$$

$$\Psi_2 = \overline{\phi}\, h. \tag{S.42b}$$

Multiplying Eq. (S.10) with $\overline{\phi}$ and adding Eq. (S.36), we obtain

$$\partial_t \Psi_1 = \mathrm{Pe}^{-1}\, \vec{\nabla}_\parallel \cdot \overline{D}_{\mathrm{eff}}\, h\, \vec{\nabla}_\parallel (1 - \overline{\phi}) - \vec{\nabla}_\parallel \cdot (1 - \overline{\phi})\, \vec{\Phi}_\parallel - \mathcal{E}\, j, \tag{S.43a}$$

$$\partial_t \Psi_2 = \mathrm{Pe}^{-1}\, \vec{\nabla}_\parallel \cdot \overline{D}_{\mathrm{eff}}\, h\, \vec{\nabla}_\parallel \overline{\phi} - \vec{\nabla}_\parallel \cdot \overline{\phi}\, \vec{\Phi}_\parallel. \tag{S.43b}$$

Here, $\Psi_1$ is the effective height of the solvent (water), and $\Psi_2$ is the effective height of the solute (1,2-propanediol). Although $h = \Psi_1 + \Psi_2$ and $\phi = \Psi_2 / h$ still have to be calculated in order to evaluate the terms in the evolution equations, it is advantageous to use the conserved quantities in the finite volumes discretization.

Equations (S.43) are discretized in an axisymmetric finite volumes scheme according to [8, 9] (non-negativity preserving numerical mobilities for hydrodynamic fluxes). Compositions on the cell edges were extrapolated by an essentially non-oscillatory third-order upwind scheme according to [10]. Here, the third order correction to the first order upwind composition is flux limited. This suppresses non-physical oscillations while minimizing numerical diffusion. We also tested a first-order upwind scheme and a central differences scheme, observing strong numerical (non-physical) diffusion and spurious oscillations, respectively.

We used a strongly graded grid where the grid spacing varies from 0.25 (in scaled units) close to the contact line to $\sim 8000$ far away from the drop. Inside the drop, the grid spacing increases to $\sim 400$.

Time integration is performed with a splitting scheme, implemented with the sundials CVode package [11], version 4.1.0. In the first substep, evaporation is applied explicitly. In the second step, the advection terms are integrated with a second order fully implicit backward differentiation (BDF) method. Importantly, capillary and Marangoni fluxes cannot be split into separate substeps as in [9], because this would lead to strong numerical dispersion. In the third substep, solute diffusion and dispersion is integrated with an implicit second order BDF method, using explicit values for the hydrodynamic fluxes from the previous substep.

With this scheme, volume conservation of the nonvolatile component was observed to be better than $V/V_0 - 1 \lesssim 10^{-6}$ over the simulated time. In terms of individual grid cells and time steps, this accuracy is around machine precision.

---


[1] M. Moosavi and A. A. Rostami, Densities, viscosities, refractive indices, and excess properties of aqueous 1,2-etanediol, 1,3-propanediol, 1,4-butanediol, and 1,5-pentanediol binary mixtures, Journal of Chemical and Engineering Data **62**, 156 (2017).

[2] J. George and N. V. Sastry, Density, dynamic viscosities, speeds of sound, and relative permittivities for water + alkanediols (propane-1,2- and -1,3-diol and butane-1,2-, -1,3-, -1,4-, and -2,3-diol) at different temperatures, Journal of Chemical and Engineering Data **48**, 1529 (2003).

[3] P. Jarosiewicz, G. Czechowski, and J. Jadżyn, The viscous properties of diols. v. 1,2-hexanediol in water and butanol solutions, Verlag der Zeitschrift für Naturforschung A **59**, 559 (2004).

[4] A. Oron, S. H. Davis, and S. G. Bankoff, Long-scale evolution of thin liquid films, Reviews of Modern Physics **69**, 931 (1997).

[5] J. Eggers and L. M. Pismen, Nonlocal description of evaporating drops, Physics of Fluids **22**, 112101 (2010).

[6] O. E. Jensen and J. B. Grotberg, The spreading of heat or soluble surfactant along a thin liquid film, Physics of Fluids A: Fluid Dynamics **5**, 58 (1993).

[7] U. Thiele, D. V. Todorova, and H. Lopez, Gradient dynamics description for films of mixtures and suspensions: Dewetting triggered by coupled film height and concentration fluctuations, Physical Review Letters **111**, 117801 (2013).

[8] J. A. Diez, L. Kondic, and A. Bertozzi, Global models for moving contact lines, Physical Review E **63**, 011208 (2000).

[9] M. Lenz, M. Rumpf, and G. Grün, A finite volume scheme for surfactant driven thin film flow, in *Proceedings of the Third International Symposium on Finite Volumes for Complex Applications*, edited by R. Herbin and D. Kröner (Hermes Penton Science, 2002) pp. 567–574.

[10] B. P. Leonard and S. Mokhtari, Beyond first-order upwinding: The ultra-sharp alternative for non-oscillatory steady-state simulation of convection, International Journal for Numerical Methods in Engineering **30**, 729 (1990).

[11] S. D. Cohen, A. C. Hindmarsh, and P. F. Dubois, CVODE, a stiff/nonstiff ODE solver in c, Computers in Physics **10**, 138 (1996).
